# Supplementary material for: Runtime Verification via Rational Monitor with Imperfect Information
Source: arXiv:2408.11627 source file (2024-08-21)
Supplement: Supplementary file 1 [file AdditionalPage.tex]

\newpage

\section{Explanation of how we dealt with reviewer's comments}

%We thank all reviewers for their comments. We tried our best to tackle them in the camera ready version of this paper.

\subsubsection{Reviewer 1}

\begin{itemize}
    \item We fixed the title as suggested by another reviewer as well.
    \item The property generation is completely random. The size of the property is, indeed, the number of temporal operators of the formula. We experimented thousands of properties. We did not count the nested operators, but the number of operators inside each formula. The number of nested operators might be an interesting feature to consider in future extensions of the work.
    \item The suggested comparison with other works is interesting. Of course, we do not have space here to carry it out, but we will definitely consider it for future versions.
\end{itemize}

\subsubsection{Reviewer 2}

\begin{itemize}
	
\item To give you the intuition about the indistinguishability, consider the following example. Suppose that the rover can send a sequence of 3 bits to the monitor and that 101 is decoded as a cut and 001 is a rust. If the monitor receives 01, it cannot determine if there is a cut or a rust. This is because the missing bit determines the event. A bit can be missed due to a connection problem or to a signal band limited (in our case limited to two bits).
%Bisogna scrivere meglio sta frase
%"Let us assume that, because of the rover’s limited resources, the latter is not always capable of sending all the information to the monitor. Because of this, sometimes the monitor is not able to distinguish a cut from a rust stain.” 
%-The causality between these two lines is unclear. Is there a way for the monitor to distinguish between a cut and a rust stain? What should the rover send?

\item The reviewer was right about the property, we actually meant $\land$ instead of $\rightarrow$. In such a way the property matches our description and is also more relevant as an example.

\item Since the standard notion of monitorability does not change w.r.t. to standard RV there is no point in discussing it in this paper. A monitorable (resp., non monitorable) property, remains monitorable (resp., non monitorable) in our setting. When imperfect information is considered, it is not that the property is not monitorable, but the result is biased by assuming wrong information. This is what our work is used for.

\item Thanks to the reviewer, we improved and fixed a bug in the implementation. Already publicly available.

\end{itemize}

\subsubsection{Reviewer 3}

%A discussion about the expressivity of indistinguishability relations in the context of "uncertainty" would help to motivate their approach and help potential users.

\begin{itemize}
    \item We updated the title as suggested. Now is more precise w.r.t. the paper's topic.

    \item The property analysed in the case study is satisfied w.r.t. a standard monitor simply because we observe $b$ and then we do not observe $c$ in the following event of the trace. A monitor should not return $?$ because the property is a liveness property, and the requirement to its satisfaction has been met (a monitor should guarantee anticipation).
    
    \item We fixed the sentences in the case study section that were pointed out. This is to better state that the indistinguishability relations is a possible way to formalise imperfect information (naturally, not the only one).
    
    \item All typos have been fixed as suggested by the reviewer.
\end{itemize}
